# Supplementary material for: EE-MLLM: A Data-Efficient and Compute-Efficient Multimodal Large Language Model
Source: arXiv:2408.11795 source file (2025-04-06)
Supplement: Supplementary file 1 [file X_suppl.tex]

\clearpage
\setcounter{page}{1}
\maketitlesupplementary
